# Supplementary material for: RCStat: A Statistical Framework for using Relative Contextualization in Transformers
Source: arXiv:2506.19549 source file (2026-10-13)

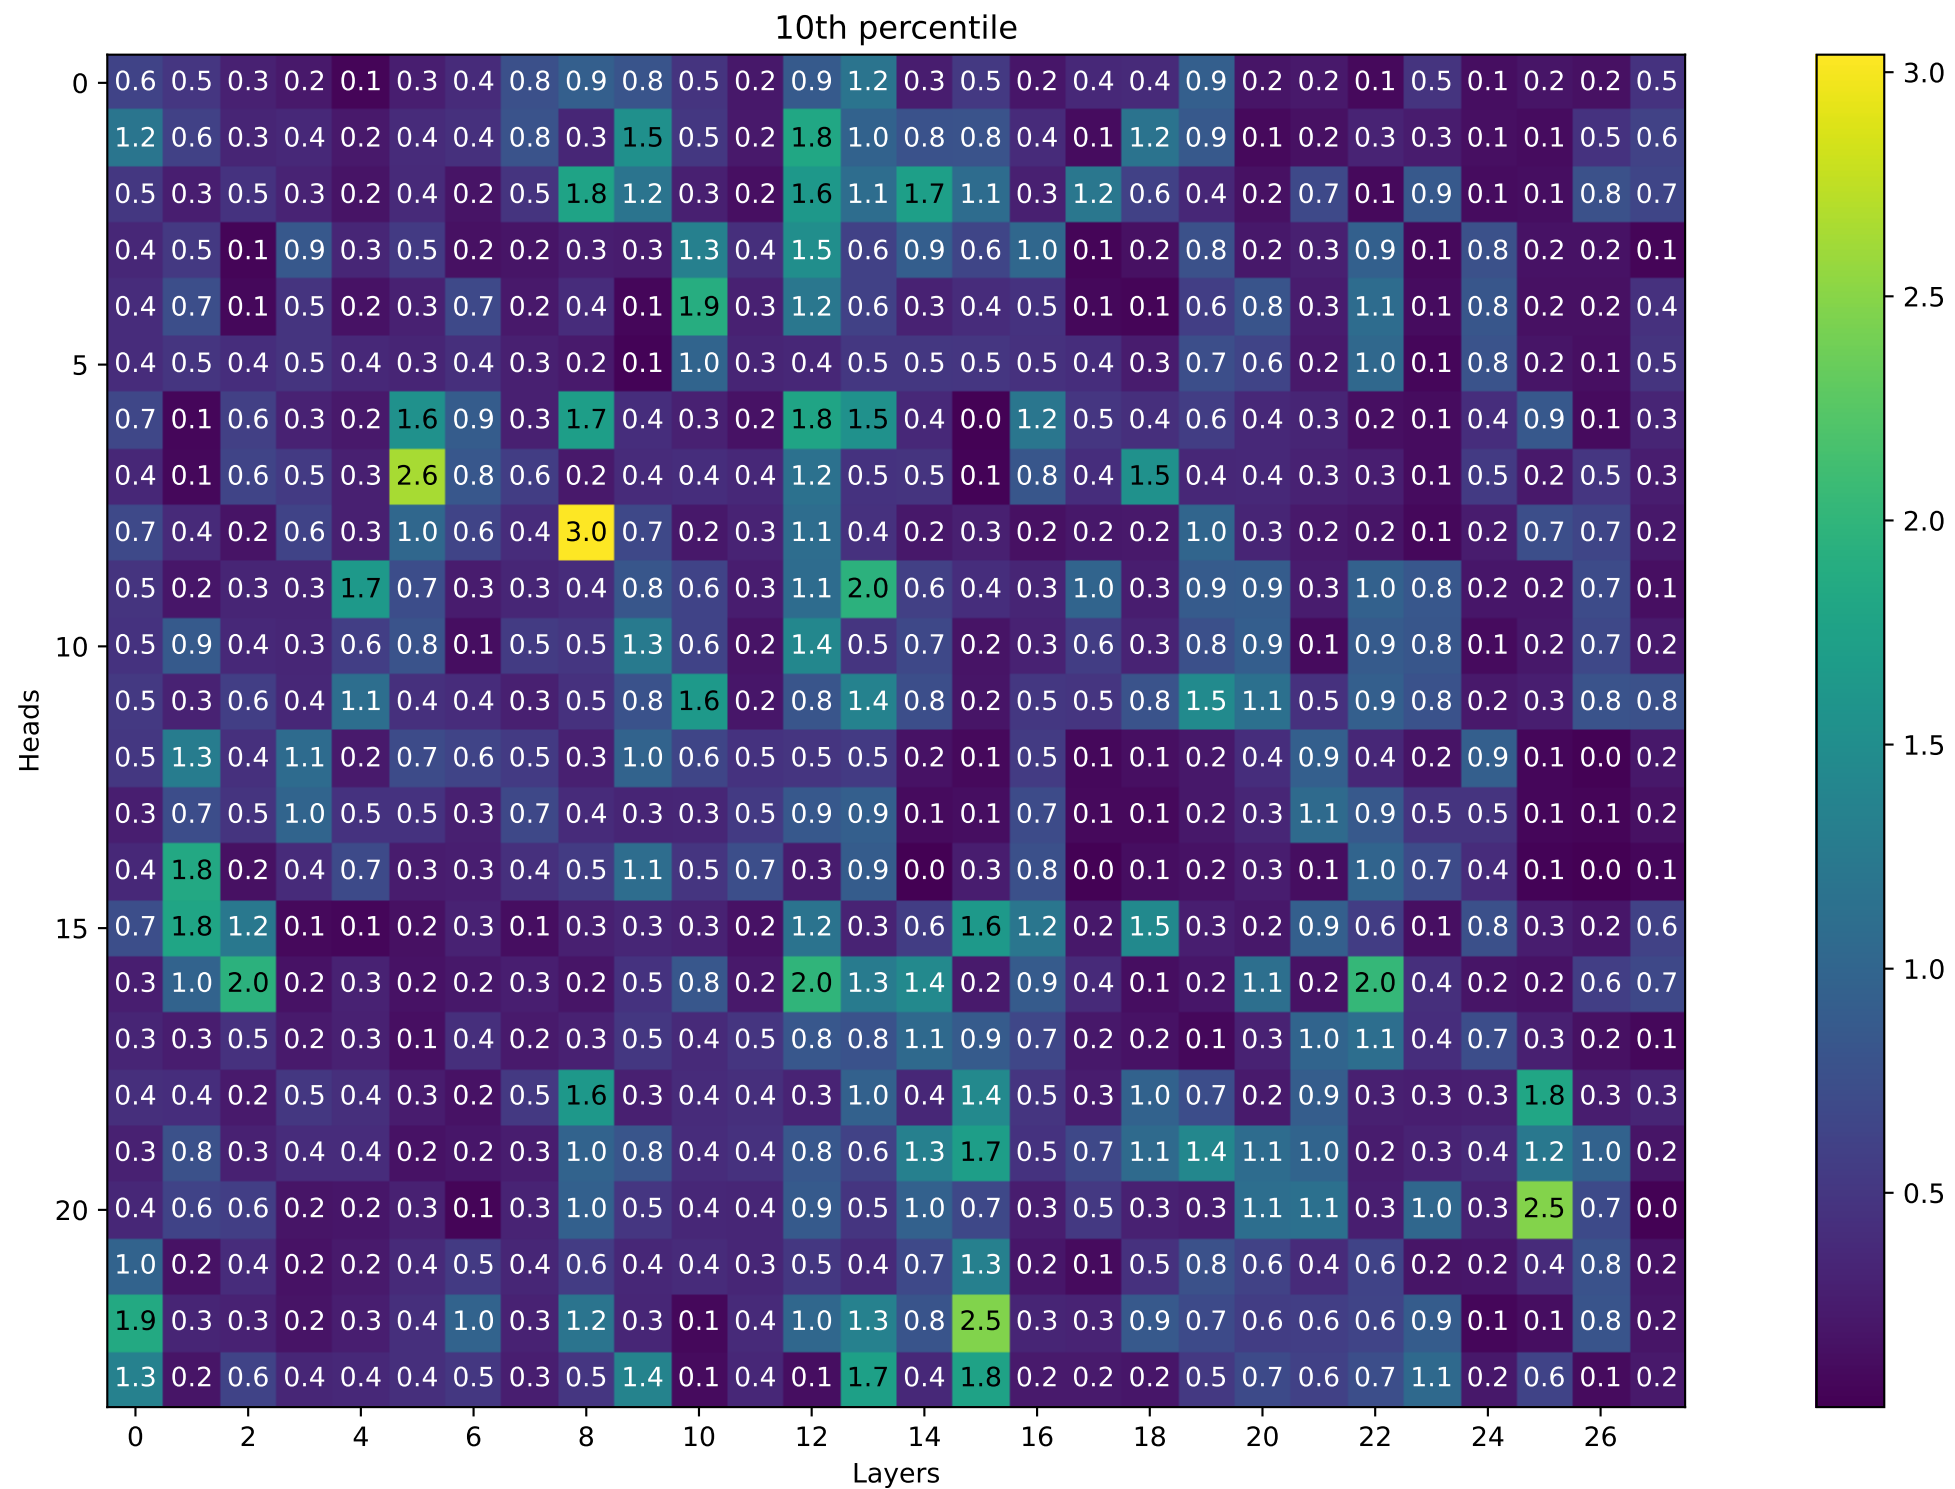

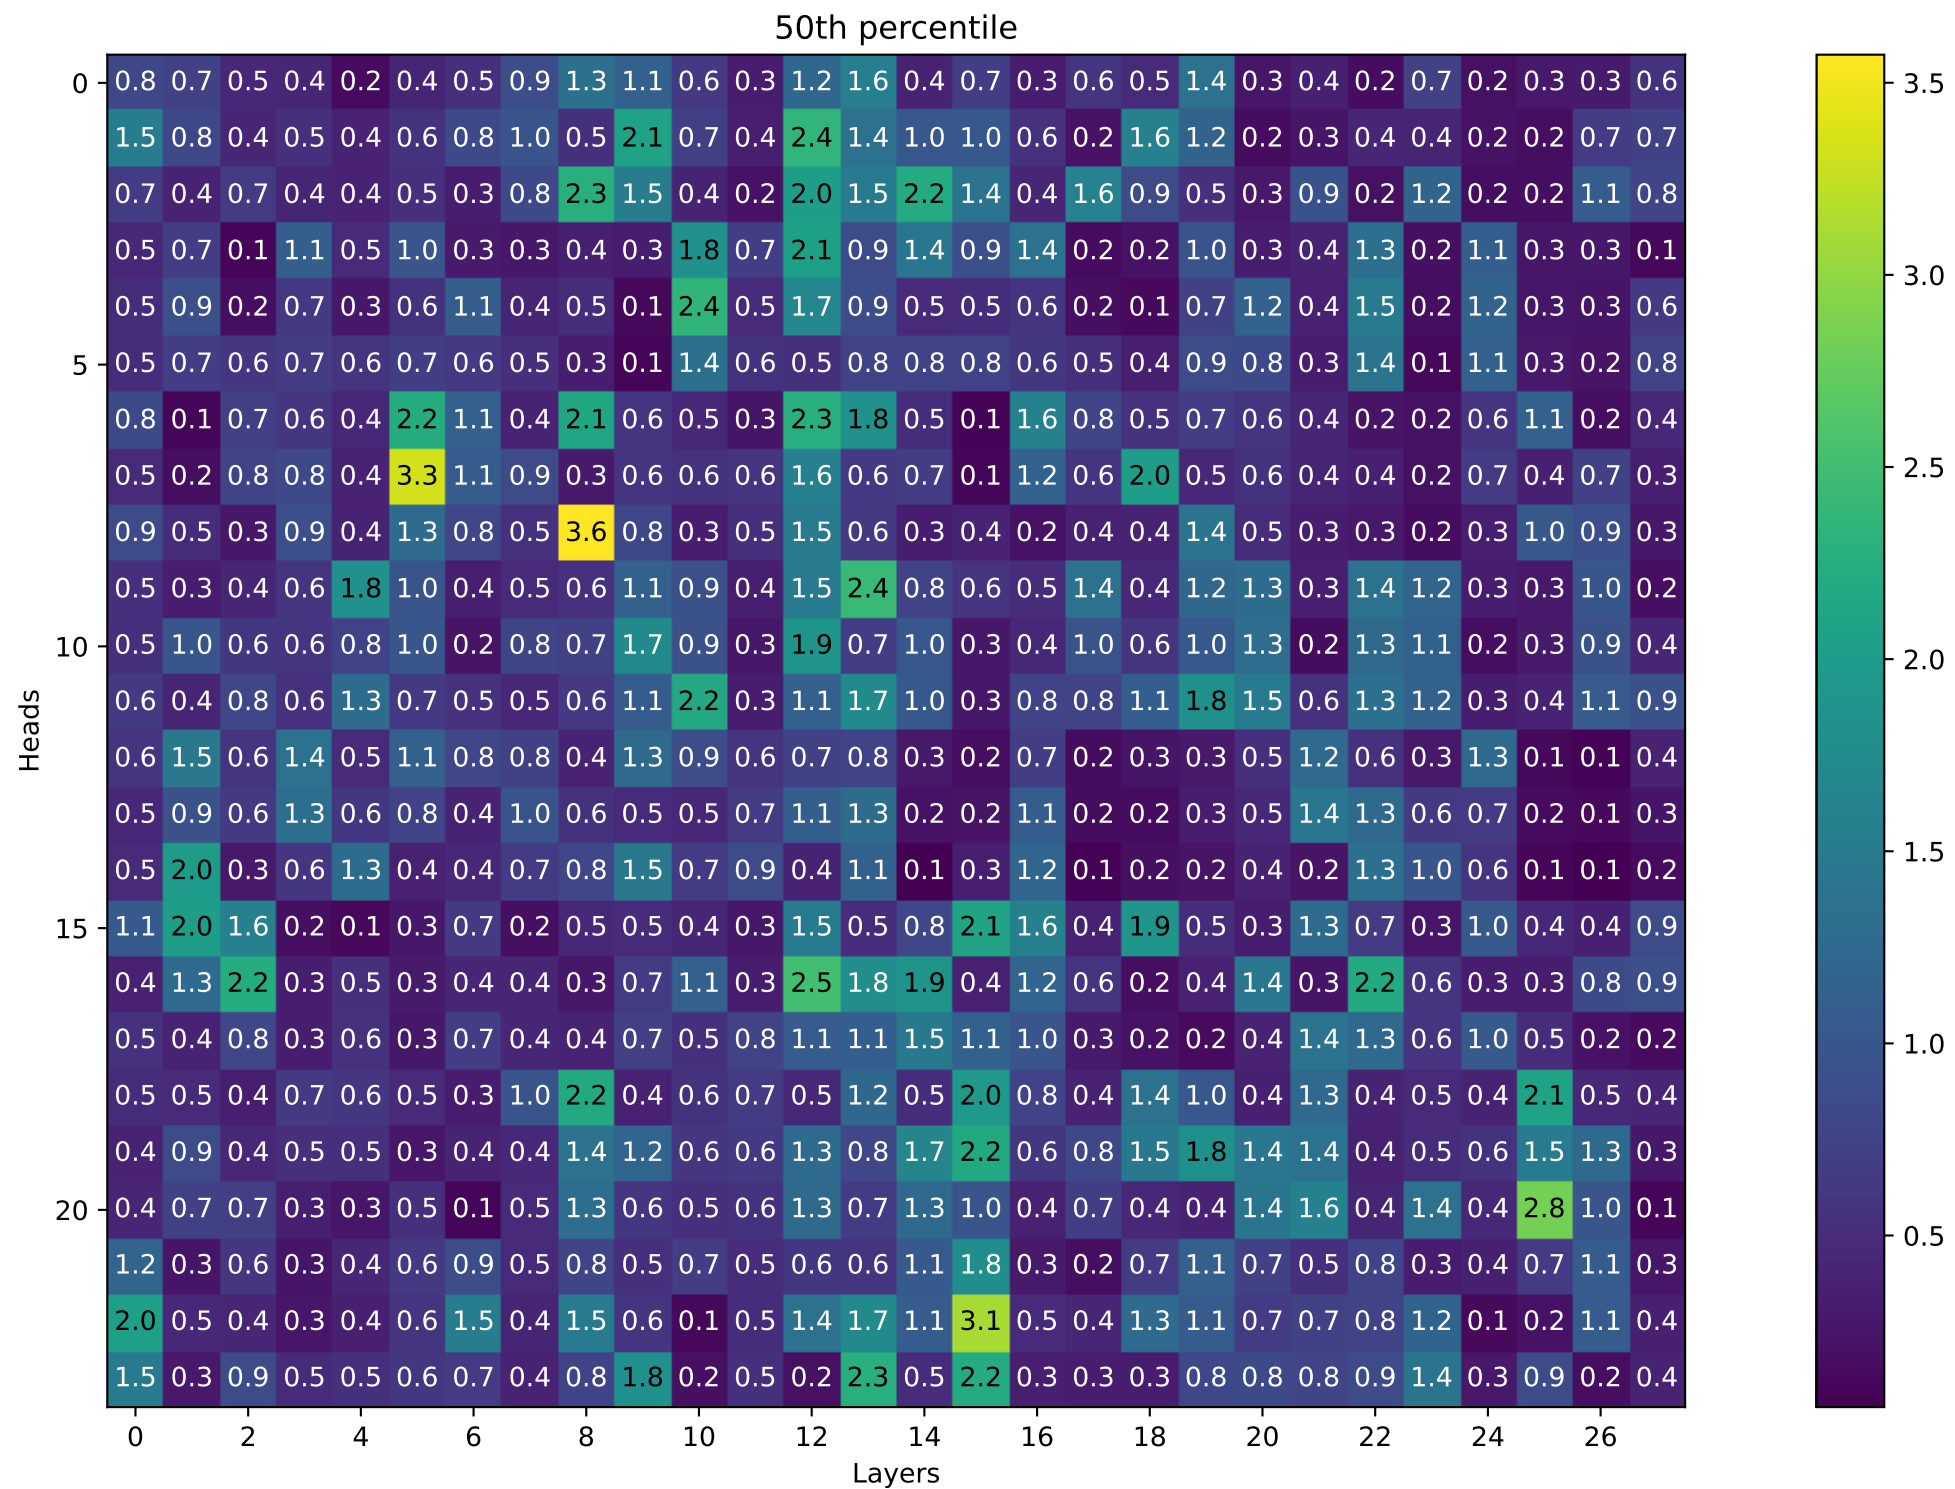

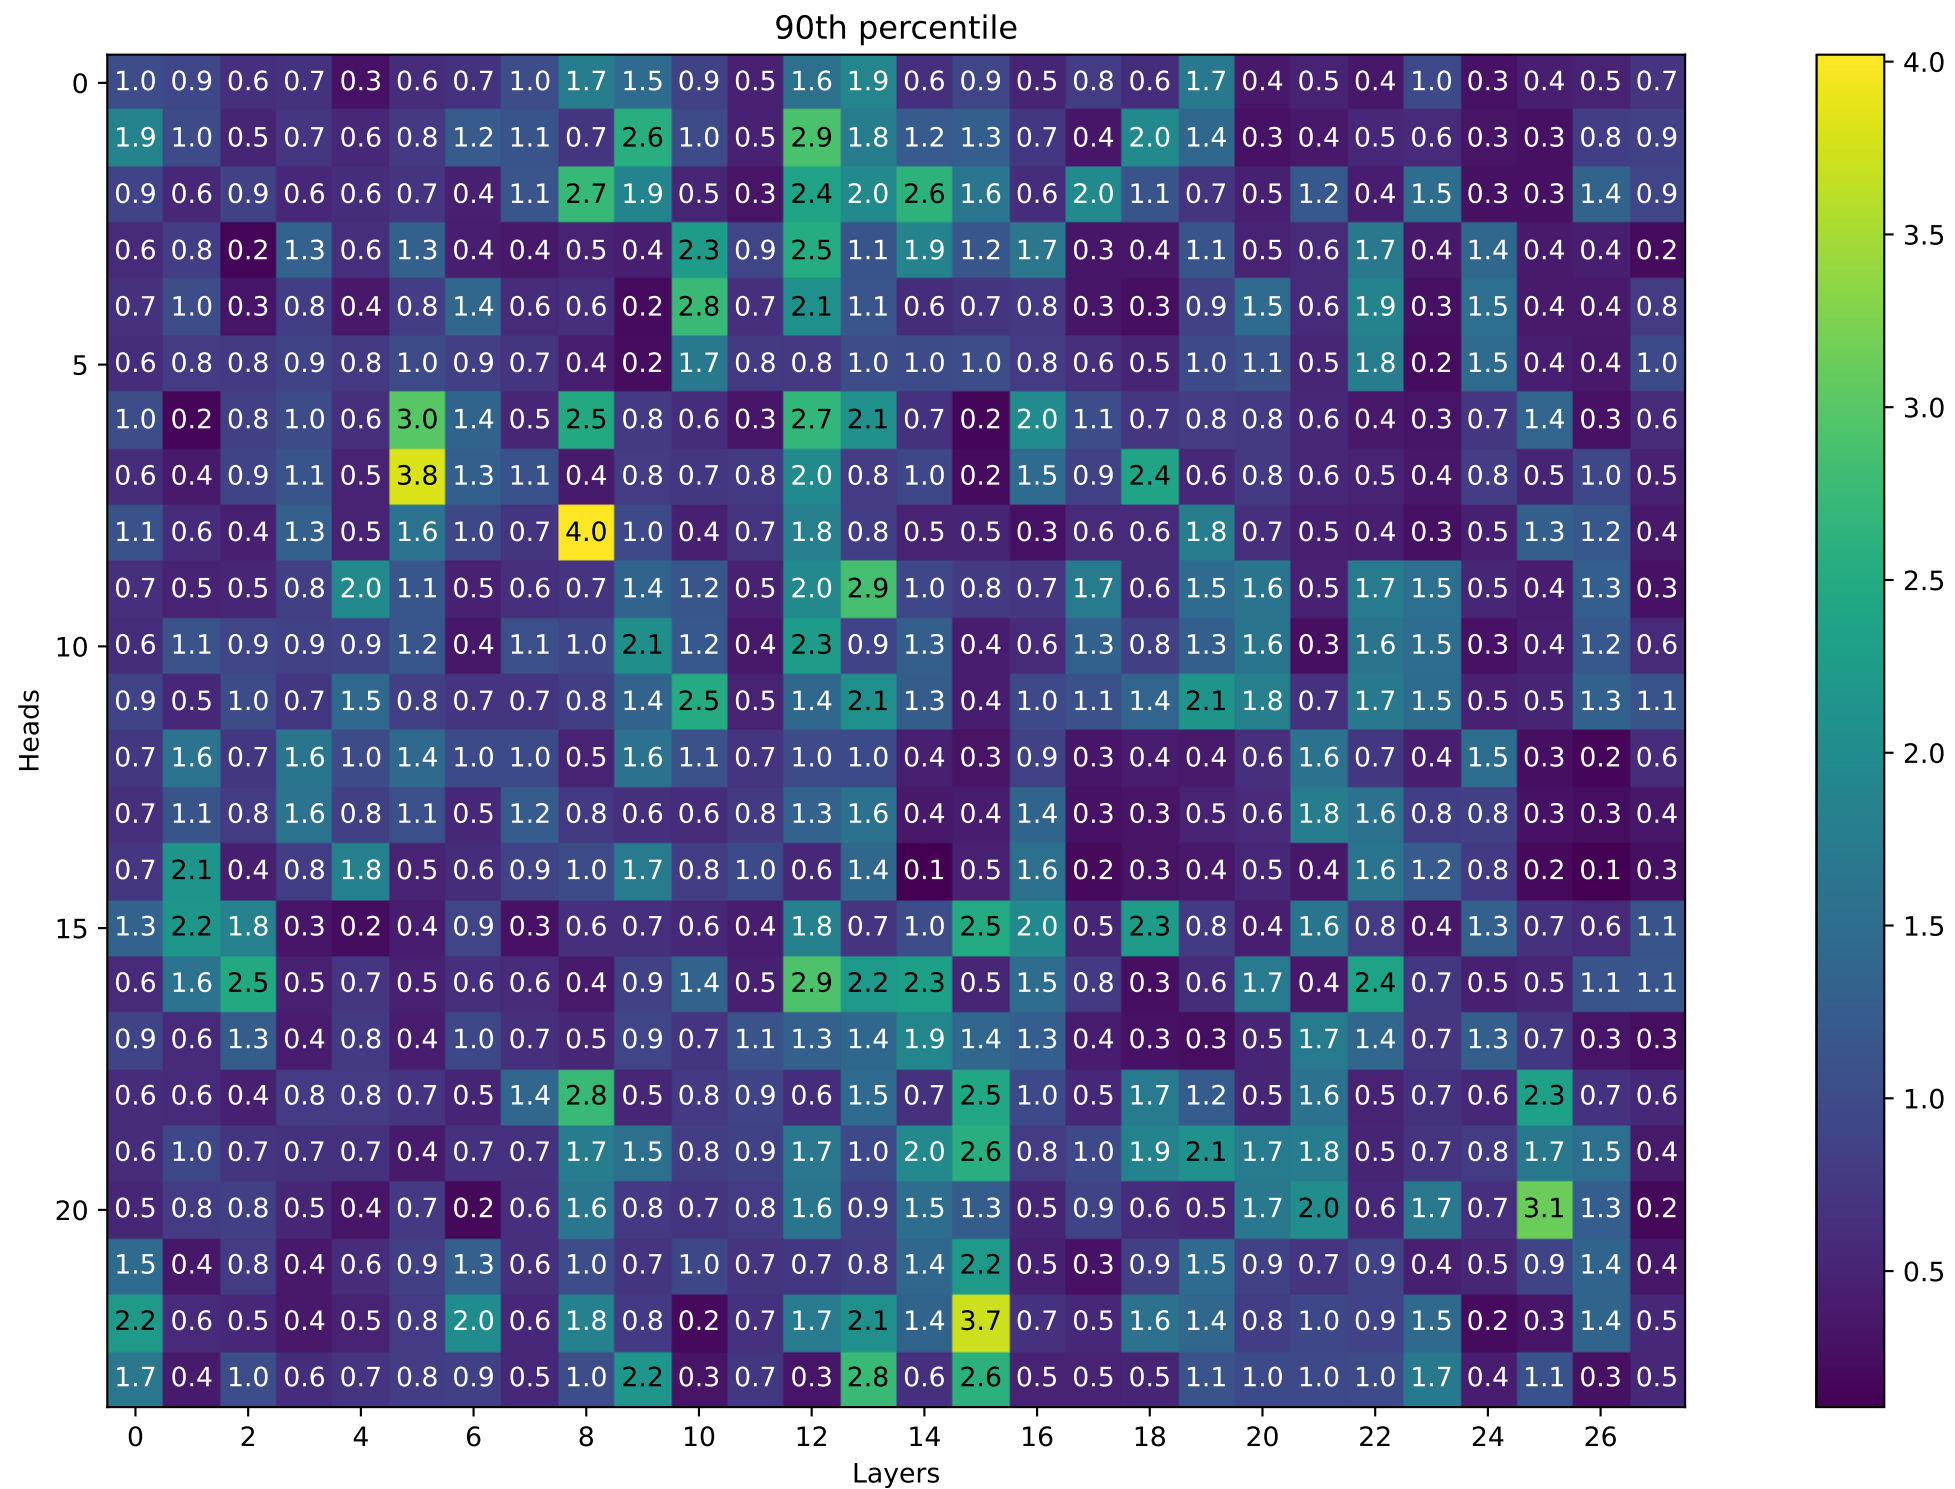

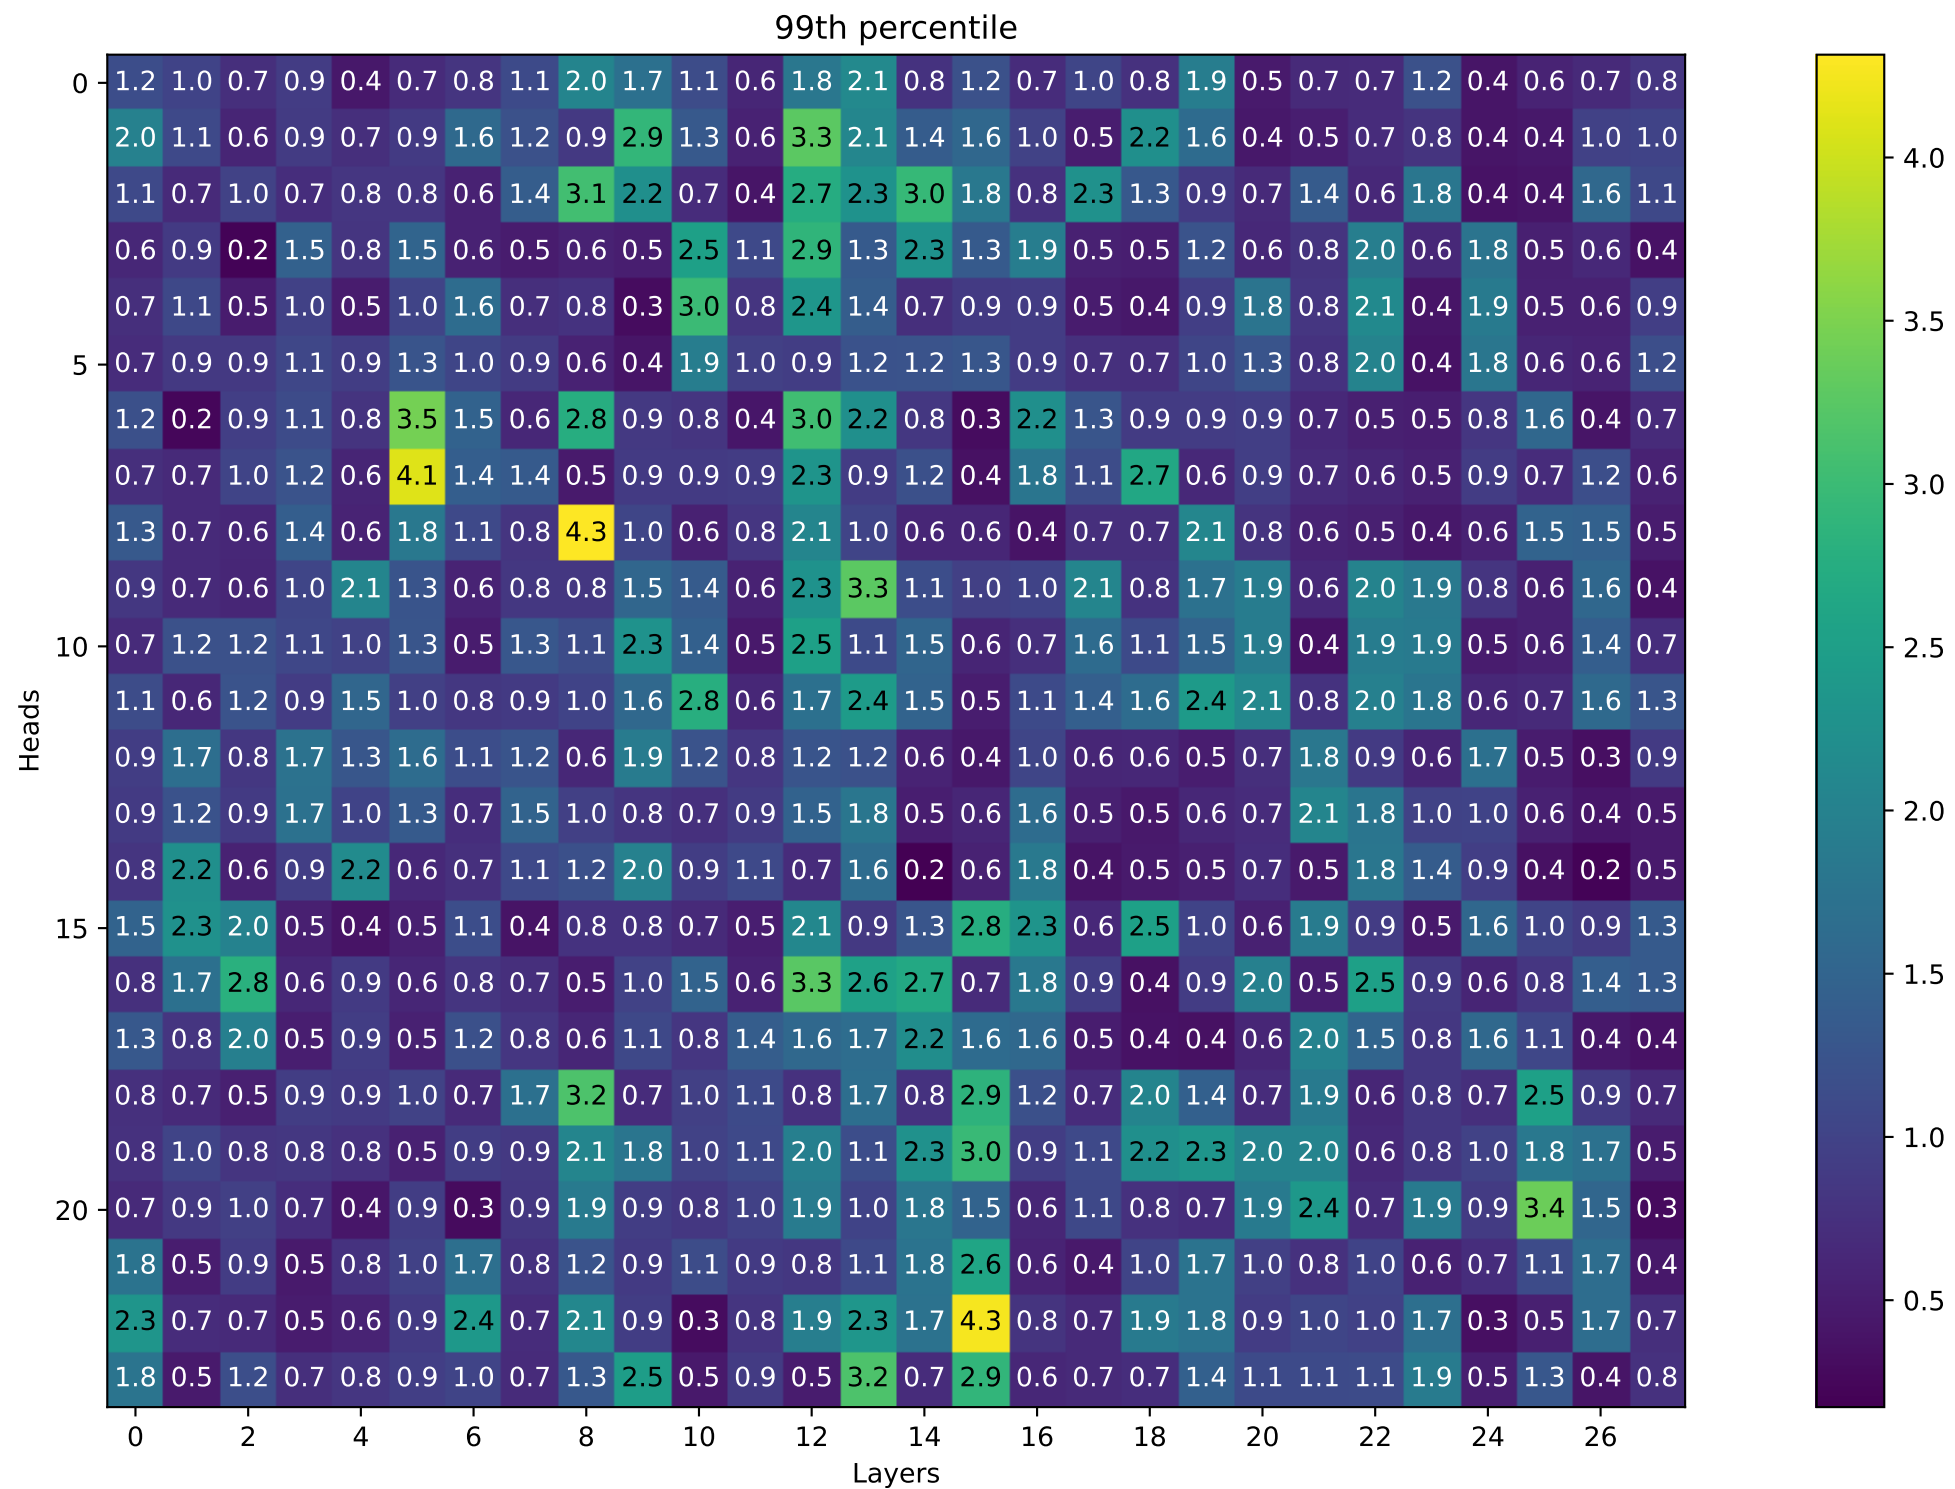

Supplement: Supplementary file 2 [file qmsum_percentile_heatmaps.pdf]
