# Supplementary material for: RCStat: A Statistical Framework for using Relative Contextualization in Transformers
Source: arXiv:2506.19549 source file (2026-10-13)
Supplement: Supplementary file 4 [file supplementary.tex]

% if you need to pass options to natbib, use, e.g.:
%     \PassOptionsToPackage{numbers, compress}{natbib}
% before loading neurips_2025

\documentclass{article}

% ready for submission
\usepackage{neurips_2025}
\usepackage{comment}

\usepackage{enumitem}
\usepackage[table]{xcolor}
\definecolor{mypink}{RGB}{255, 192, 203}
\definecolor{mygreen}{RGB}{144, 238, 144}

% to compile a preprint version, e.g., for submission to arXiv, add add the
% [preprint] option:
%     \usepackage[preprint]{neurips_2025}

% to compile a camera-ready version, add the [final] option, e.g.:
    % \usepackage[final]{neurips_2025}

% to avoid loading the natbib package, add option nonatbib:
%    \usepackage[nonatbib]{neurips_2025}

% Recommended, but optional, packages for figures and better typesetting:
\usepackage{microtype}
\usepackage{graphicx}
\usepackage{subcaption}
\usepackage{booktabs} % for professional tables
\usepackage{multirow}

% hyperref makes hyperlinks in the resulting PDF.
% If your build breaks (sometimes temporarily if a hyperlink spans a page)
% please comment out the following usepackage line and replace
% \usepackage{icml2024} with \usepackage[nohyperref]{icml2024} above.
\usepackage{hyperref}

% Attempt to make hyperref and algorithmic work together better:

% Use the following line for the initial blind version submitted for review:
% \usepackage{icml2024}

% If accepted, instead use the following line for the camera-ready submission:
% \usepackage[accepted]{icml2024}

% For theorems and such
\usepackage{amsmath}
\usepackage{amssymb}
\usepackage{mathtools}
\usepackage{amsthm}
\usepackage{algorithm}
\usepackage[noend]{algpseudocode}
\usepackage{wrapfig}

\usepackage{graphicx}
\graphicspath{{./Figures/}}
% if you use cleveref..
\usepackage[capitalize,noabbrev]{cleveref}

%%%%%%%%%%%%%%%%%%%%%%%%%%%%%%%%
% THEOREMS
%%%%%%%%%%%%%%%%%%%%%%%%%%%%%%%%
\theoremstyle{plain}

\theoremstyle{definition}

\theoremstyle{remark}

% Todonotes is useful during development; simply uncomment the next line
%    and comment out the line below the next line to turn off comments
%\usepackage[disable,textsize=tiny]{todonotes}
\usepackage[textsize=tiny]{todonotes}

\usepackage[table]{xcolor}
\usepackage{colortbl} % Optional if xcolor[table] is loaded

% Define a light green color
\definecolor{lightgreen}{RGB}{220, 255, 220}  % You can tweak RGB values

% The \icmltitle you define below is probably too long as a header.
% Therefore, a short form for the running title is supplied here:
% \icmltitlerunning{KV Cache Reuse in RAG Applications}
% \title{A Statistical Gauge of Contextualization in Transformer Models}
% \title{Gauge Me If You Can: Statistical Tools for Tracking Context in Transformers}
% \title{A Statistical Tool of Relativity \\ in LLM Contextualization}
% \title{A Statistical Tool for Measuring Contextualization via Pre-Softmax Attention}
% \title{RCStat: A Statistical Gauge of Contextualization via Attention Logits}
\title{Supplementary: \textsc{RCStat}: A Statistical Framework for using Relative Contextualization in Transformers} 
% via Raw Attention Logits
% \title{Statistical Tools for Measuring Contextualization\\ in Auto-Regressive Transformer}
% \title{}
%\title{SogftA Statistical Tool of Relativity in Contextualization \\ of Auto-Regressive Transformer}

% \title{A Statistical Tool for Gauging the Relativity of \\Contextualization in Auto-Regressive Transformers}
% \title{Softmax is not }

\author{%
  Debabrata Mahapatra\thanks{Use footnote for providing further information
    about author (webpage, alternative address)---\emph{not} for acknowledging
    funding agencies.} \\
  Adobe Research\\
  Bangalore, India \\
  \texttt{dmahapatra@adobe.com}\\
  % examples of more authors
  \And
  Shubham Agarwal \\
  % Affiliation \\
  Adobe Research\\
  Bangalore, India\\
  \texttt{shagarw@adobe.com}\\
  \AND
  Apoorv Saxena \\
  Adobe Research\\
  Bangalore, India \\
  \texttt{apoorvs@adobe.com}\\
  \AND
  Subrata Mitra \\
  Adobe Research\\
  Bangalore, India \\
  \texttt{sumitra@adobe.com}\\
  % \And
  % Coauthor \\
  % Affiliation \\
  % Address \\
  % \texttt{email} \\
  % \And
  % Coauthor \\
  % Affiliation \\
  % Address \\
  % \texttt{email} \\
}

\begin{document}
\maketitle
\input{suppl}
\end{document}
